# Supplementary material for: Sinkhorn Natural Gradient for Generative Models
Source: arXiv:2011.04162 source file (2020-11-09)
Supplement: Supplementary file 1 [file appendix_copy.tex]

\section{Proof of Theorem \ref{theorem_consistency}}
%\begin{theorem}[Theorem \ref{theorem_consistency} restated]
%\begin{equation}
%\bar \HB(\theta^t) \rightarrow \HB(\theta^t),\ \mathrm{as}\ n\rightarrow \infty
%\end{equation}
%\end{theorem}

%Denote $\AM[f, \alpha](\cdot) = \softmin_{x\sim\alpha} c(x, \cdot) - f(x)$ and 
Denote $A[u, \alpha] = \int_\XM k(x, y) u(x)\dB\alpha(x)$ with $k(x, y) = \exp(-\frac{c(x, y)}{\gamma})$ and recall the definition of the Sinkhorn mapping \eqref{eqn_sinkhorn_mapping}.
We have $\AM[f, \alpha] = -\gamma\log A[e^{f/\gamma},\alpha]$.

%Denote $\GM(\alpha) = \OTgamma(\alpha, \beta)$.
%\begin{equation}
%	\GM(\alpha) = \max_{f\in\CM(\XM)} \left\{\HM(f, \alpha) \defi \langle f, \alpha\rangle + \langle\AM[f, \alpha], \beta\rangle\right\}
%\end{equation}
%Denote $\FM[\alpha] = f_\alpha$.
%\begin{theorem}
%	$\FM[\alpha]$ is continuous with respect to $\alpha$:
%	For any sequence $\alpha^n\rightarrow \alpha$, we have
%	\begin{equation}
%		\|\lim_{n\rightarrow \infty}\FM[\alpha^n] - \FM[\alpha]\|_\infty = 0.
%	\end{equation}
%\end{theorem}


Let $\bar g\in\CM(\XM)$ be a perturbation to $\bar f$. We compute that for a fixed measure $\kappa$
\begin{equation}\label{eqn_Gateaux_derivative}
	D_1\AM[\bar f, \kappa][\bar g] = \frac{\int_\XM\exp\left(-\frac{1}{\gamma}(c(x, y) - \bar f(x))\right)\bar g(x)\dB\kappa(x)}{\int_\XM\exp\left(-\frac{1}{\gamma}(c(x, y) - \bar f(x))\right)\dB\kappa(x)}.
\end{equation}
Note that 
\begin{equation}\label{eqn_proof_bound_0}
\|D_1\AM[\bar f, \kappa][\bar g]\|_\infty \leq \|\frac{\int_\XM\exp\left(-\frac{1}{\gamma}(c(x, y) - \bar f(x))\right)\dB\kappa(x)}{\int_\XM\exp\left(-\frac{1}{\gamma}(c(x, y) - \bar f(x))\right)\dB\kappa(x)}\|_\infty\cdot\|\bar g\|_\infty = \|\bar g\|_\infty.
\end{equation}
\begin{theorem} \label{theorem_continuity}
	$D_1f(\theta, \mu)$ is Lipschitz continuous with respect to $\mu$ under the operator norm: 
	\begin{equation}
		\|D_1f(\theta, \mu) - D_1f(\theta, \mu')\|_{op} = \OM(d_{bl}(\mu, \mu')).
	\end{equation}	
\end{theorem}
\section{Proof of Theorem \ref{theorem_continuity}}
	The optimality of the Sinkhorn potential $f(\theta, \mu)$ can be restated as
	\begin{equation}
		f(\theta, \mu) = \BM\left[f(\theta, \mu), \theta, \mu\right],
	\end{equation}
	where we recall the definition of $\BM$ in \eqref{eqn_main_fix_point}
	\begin{equation}
		\BM\left[f, \theta, \mu\right] = \AM\left[\AM\left[f, {T_{\theta}}_\sharp \mu\right], \beta\right].
	\end{equation}
	By repeating this fixed point iteration $l = \lceil\log_{\lambda}\frac{1}{3}\rceil/2$ times, we then have 
	\begin{equation}
		f(\theta, \mu) = \EM[f(\theta, \mu), \theta],
	\end{equation}
	where $\EM[f(\theta, \mu), \theta] = \BM[\cdots\BM[f, \theta]]$ is the $l$ times composition of $\BM$ in its first variable.
%	Note that in $\BM[\cdot,\cdot,\cdot]$ we drop the dependence on the fixed measure $\beta$.
	Assume $c(x, y)\leq M_c$, $\forall x, y \in\XM$ and let $\lambda = \frac{e^{M_c/\gamma} - 1}{e^{M_c/\gamma} + 1}$.
	Then for arbitrary measure $\alpha\in\MM_1^+(\XM)$, we have from \eqref{eqn_contraction_EM}
	\begin{equation}\label{eqn_contraction_of_A}
		||D^1\EM[f, \theta]\|_{op} \leq \frac{2}{3},
	\end{equation}
	where for a (linear) operator $\CM:\CM(\XM)\rightarrow\CM(\XM)$, $\|\CM\|_{op} \defi \max_{f\in\CM(\XM)} \frac{\|\CM f\|_\infty}{\|f\|_\infty}$.

	Let $h$ be a bounded perturbation to $\theta$, i.e $\|h\|_\infty \leq M_h$.
	Using the chain rule of Gateaux derivative, we derive
	\begin{equation}
		d^1_hf(\theta, \mu) = d^1_{d^1_{h}f(\theta, \mu)}\BM[f(\theta, \mu), \theta, \mu] + d^2_{h}\BM[f(\theta, \mu), \theta, \mu].
	\end{equation}
	Denote $f_{\theta, \mu} \defi f(\theta, \mu)$.
	\begin{equation} \label{eqn_proof_main}
	\begin{aligned}
	& \|d^1_hf_{\theta, \mu} - d^1_hf_{\theta, \mu'}\|_\infty\\
	\leq\quad & \|d^1_{d^1_{h}f_{\theta, \mu}}\BM[f_{\theta, \mu}, \theta, \mu]  - d^1_{d^1_{h}f_{\theta, \mu'}}\BM[f_{\theta, \mu'}, \theta, \mu']\|_\infty +  \|d^2_{h}\BM[f_{\theta, \mu}, \theta, \mu] - d^2_{h}\BM[f_{\theta, \mu'}, \theta, \mu']\|_\infty\\
	\leq\quad & \underbrace{\|d^1_{d^1_{h}f_{\theta, \mu}}\BM[f_{\theta, \mu}, \theta, \mu]  - d^1_{d^1_{h}f_{\theta, \mu'}}\BM[f_{\theta, \mu}, \theta, \mu]\|_\infty}_{\textcircled{1}} + \underbrace{\|d^1_{d^1_{h}f_{\theta, \mu'}}\BM[f_{\theta, \mu}, \theta, \mu]  - d^1_{d^1_{h}f_{\theta, \mu'}}\BM[f_{\theta, \mu'}, \theta, \mu]\|_\infty}_{\textcircled{2}} \\
	\quad& + \underbrace{\|d^1_{d^1_{h}f_{\theta, \mu'}}\BM[f_{\theta, \mu'}, \theta, \mu]  - d^1_{d^1_{h}f_{\theta, \mu'}}\BM[f_{\theta, \mu'}, \theta, \mu']\|_\infty}_{\textcircled{3}} + \underbrace{\|d^2_{h}\BM[f_{\theta, \mu}, \theta, \mu] - d^2_{h}\BM[f_{\theta, \mu'}, \theta, \mu']\|_\infty}_{\textcircled{4}}.
	\end{aligned}
	\end{equation}
	The following subsections analyze $\textcircled{1}$ to $\textcircled{4}$ individually. In summary, we have
	\begin{equation}
		\textcircled{1} \leq 4\lambda^2 \|d^1_{h}f_{\theta, \mu} - d^1_{h}f_{\theta, \mu'}\|_\infty,
	\end{equation}
	and \textcircled{2}, \textcircled{3}, \textcircled{4} are all of order $\OM(d_{bl}(\mu, \mu'))$.
	Therefore we conclude
	\begin{equation}
		(1-4\lambda^2)\|d^1_{h}f_{\theta, \mu} - d^1_{h}f_{\theta, \mu'}\|_\infty = \OM(d_{bl}(\mu, \mu')) \Rightarrow \|d^1_{h}f_{\theta, \mu} - d^1_{h}f_{\theta, \mu'}\|_\infty = \OM(d_{bl}(\mu, \mu')).
	\end{equation}
	
	\subsection{Bounding \textcircled{1}}
	For $\textcircled{1}$, observe that
	\begin{align*}
		\|d^1_{d^1_{h}f_{\theta, \mu}}\BM[f_{\theta, \mu}, \theta, \mu]  - d^1_{d^1_{h}f_{\theta, \mu'}}\BM[f_{\theta, \mu'}, \theta, \mu]\|_\infty =\ & \|D^1\BM[f_{\theta, \mu}, \theta, \mu](d^1_{h}f_{\theta, \mu} - d^1_{h}f_{\theta, \mu'})\|_\infty \\
		\leq\ & \|D^1\BM[f_{\theta, \mu}, \theta, \mu]\|_{op}\|d^1_{h}f_{\theta, \mu} - d^1_{h}f_{\theta, \mu'}\|_\infty \\
		\leq\ & 4\lambda^2 \|d^1_{h}f_{\theta, \mu} - d^1_{h}f_{\theta, \mu'}\|_\infty.
	\end{align*}
	
	\subsection{Bounding \textcircled{2}}
	Denote $k(x, y) = \exp(-\frac{c(x, y)}{\gamma})$. The expression \eqref{eqn_Gateaux_derivative} allow us to compute for two function $\bar f$ and $\bar f'$
	\begin{align*}
	&\|d^1_{\bar g}\AM(\bar f, \kappa) - d^1_{\bar g}\AM(\bar f', \kappa)\|_\infty\\
	=\ &\|\frac{\int_\XM k(x, y)\exp\left(\frac{\bar f(x)}{\gamma}\right)\bar g(x)\dB\kappa(x)}{\int_\XM k(x, y)\exp\left(\frac{\bar f(x)}{\gamma}\right)\dB\kappa(x)} - \frac{\int_\XM k(x, y)\exp\left(\frac{\bar f'(x)}{\gamma}\right)\bar g(x)\dB\kappa(x)}{\int_\XM k(x, y)\exp\left(\frac{\bar f'(x)}{\gamma}\right)\dB\kappa(x)}\|_\infty\\
	=\ &\|\frac{\int_{\XM^2}k(x, y)k(x', y)\left[\exp\left(\frac{\bar f(x) + \bar f'(x')}{\gamma}\right) - \exp\left(\frac{\bar f(x') + \bar f'(x)}{\gamma}\right)\right]\bar g(x)\dB\kappa(x)\dB\kappa(x')}{\int_\XM k(x', y)\exp\left(\frac{\bar f(x')}{\gamma}\right)\dB\kappa(x')\int_\XM k(x', y)\exp\left(\frac{\bar f'(x')}{\gamma}\right)\dB\kappa(x')}\|_\infty \\
	=\ &\|\frac{\int_{\XM^2}k(x, y)k(x', y)v(x, x')\left(\bar f(x) + \bar f'(x') - (\bar f(x') + \bar f'(x))\right)\bar g(x)\dB\kappa(x)\dB\kappa(x')}{\gamma\int_\XM k(x', y)\exp\left(\frac{\bar f(x')}{\gamma}\right)\dB\kappa(x')\int_\XM k(x', y)\exp\left(\frac{\bar f'(x')}{\gamma}\right)\dB\kappa(x')}\|_\infty\\
	\leq\ & \frac{2}{\gamma}\underbrace{\|\frac{\int_{\XM^2}k(x, y)k(x', y)v(x, x')\bar g(x)\dB\kappa(x)\dB\kappa(x')}{\int_\XM k(x', y)\exp\left(\frac{\bar f(x')}{\gamma}\right)\dB\kappa(x')\int_\XM k(x', y)\exp\left(\frac{\bar f'(x')}{\gamma}\right)\dB\kappa(x')}\|_\infty}_{\textcircled{a}}\cdot\|\bar f - \bar f'\|_\infty\cdot\|g\|_\infty.
	\end{align*}
	Here $v(x, x') \in [\exp\left(\frac{\bar f(x) + \bar f'(x')}{\gamma}\right), \exp\left(\frac{\bar f(x') + \bar f'(x)}{\gamma}\right)]$ is from the mean value theorem.
%	Recall that \red{$f_{\theta, \mu}$ is continuous with respect to $\mu$ and $\|g\|_\infty$ is bounded.} 
	Note that $\textcircled{a}$ is also bounded.
	Consequently, we have
	\begin{equation}\label{eqn_proof_bound_2}
		\|d^1_{\bar g}\AM(\bar f, \kappa) - d^1_{\bar g}\AM(\bar f', \kappa)\|_\infty = \OM(\|\bar f - \bar f'\|_\infty\cdot\|\bar g\|_\infty).
	\end{equation}

	We are now ready to bound \textcircled{2}.
	Denote $\alpha = {T_{\theta}}_\sharp \mu$, $g = d^1_{h}f_{\theta, \mu'}$, $f \defi f_{\theta, \mu}$ and $f' \defi f_{\theta, \mu'}$.
	Using the chain rule of Gateaux derivative we derive
	\begin{align*}
	\textcircled{2} =\ & \|d^1_{d^1_g\AM(f, \alpha)}\AM(\AM(f,\alpha), \beta) - d^1_{d^1_g\AM(f', \alpha)}\AM(\AM(f',\alpha), \beta)\|_\infty \\
	\leq\ & \underbrace{\|d^1_{d^1_g\AM(f, \alpha)}\AM(\AM(f,\alpha), \beta) - d^1_{d^1_g\AM(f', \alpha)}\AM(\AM(f,\alpha), \beta)\|_\infty}_{\textcircled{2}_1} \\
	&+ \underbrace{\|d^1_{d^1_g\AM(f', \alpha)}\AM(\AM(f,\alpha), \beta) - d^1_{d^1_g\AM(f', \alpha)}\AM(\AM(f',\alpha), \beta)\|_\infty}_{\textcircled{2}_2}
	\end{align*}
	We bound these two terms individually. First note that
	\begin{equation}
	{\textcircled{2}_1} \leq \|D^1\AM(\AM(f,\alpha), \beta)\|_{op} \underbrace{\|d^1_g\AM(f, \alpha) - d^1_g\AM(f', \alpha)\|_\infty}_{\textcircled{2}_{11}}.
	\end{equation}
	The first term is bounded by $2\lambda$ from \eqref{eqn_contraction_of_A} and the second term $\textcircled{2}_{11}$ can be bounded using \eqref{eqn_proof_bound_2}:
	Choose $\kappa = \alpha$, $\bar g=d^1_{h}f_{\theta, \mu'}$, $\bar f = f_{\theta, \mu}$ and $\bar f' = f_{\theta, \mu'}$. We have
	\begin{equation}
		\textcircled{2}_{11} = \OM(\|f_{\theta, \mu} - f_{\theta, \mu'}\|_\infty\cdot\|d^1_{h}f_{\theta, \mu'}\|_\infty) = \OM(d_{bl}(\mu, \mu')),
	\end{equation}
	where the last equality is due to the facts that $f_{\theta, \mu}$ is continuous with respect to $\mu$ and $\|d^1_{h}f_{\theta, \mu'}\|_\infty$ is bounded.
	This allows us to obtain
	\begin{equation}
		\textcircled{2}_1 = \OM(d_{bl}(\mu, \mu')).
	\end{equation}
	To bound ${\textcircled{2}_2}$, we can use the same idea as for ${\textcircled{2}_{11}}$:
	Choose $\kappa = \beta$, $\bar g=d^1_g\AM(f', \alpha)$, $\bar f = \AM(f, \alpha)$ and $\bar f' = \AM(f', \alpha)$.
	We bound
	\begin{equation}
		\textcircled{2}_2 = \OM(\|\AM(f, \alpha) - \AM(f', \alpha)\|_\infty\cdot\|d^1_g\AM(f', \alpha)\|_\infty) = \OM(\|f - f'\|_\infty\cdot\|d^1_g\AM(f', \alpha)\|_\infty) = \OM(d_{bl}(\mu, \mu')),
	\end{equation}
	where in the last equality we use the facts that $f_{\theta, \mu}$ is continuous with respect to $\mu$ and $\|d^1_g\AM(f', \alpha)\|_\infty \leq \|g\|_\infty$.
	All together we have $\textcircled{2} = \OM(d_{bl}(\mu, \mu'))$.
	\subsection{Bounding \textcircled{3}}
	Denote $k(x, y) = \exp(-\frac{c(x, y)}{\gamma})$. The expression \eqref{eqn_Gateaux_derivative} allow us to compute for two measures $\kappa$ and $\kappa'$
	\begin{align*}
		&\ \|d^1_{\bar g}\AM(\bar f, \kappa) - d^1_{\bar g}\AM(\bar f, \kappa')\|_\infty \\
		=&\ \|\frac{\int_\XM k(x, y)\exp\left(\frac{\bar f(x)}{\gamma}\right)\bar g(x)\dB\kappa(x)}{\int_\XM k(x, y)\exp\left(\frac{\bar f(x)}{\gamma}\right)\dB\kappa(x)} - \frac{\int_\XM k(x, y)\exp\left(\frac{\bar f(x)}{\gamma}\right)\bar g(x)\dB\kappa'(x)}{\int_\XM k(x, y)\exp\left(\frac{\bar f(x)}{\gamma}\right)\dB\kappa'(x)}\|_\infty\\
		\leq&\ \|\frac{\int_\XM k(x, y)\exp\left(\frac{\bar f(x)}{\gamma}\right)\bar g(x)\dB\kappa(x)}{\int_\XM k(x, y)\exp\left(\frac{\bar f(x)}{\gamma}\right)\dB\kappa(x)} - \frac{\int_\XM k(x, y)\exp\left(\frac{\bar f(x)}{\gamma}\right)\bar g(x)\dB\kappa(x)}{\int_\XM k(x, y)\exp\left(\frac{\bar f(x)}{\gamma}\right)\dB\kappa'(x)}\|_\infty \\
		&\ + \|\frac{\int_\XM k(x, y)\exp\left(\frac{\bar f(x)}{\gamma}\right)\bar g(x)\dB\kappa(x)}{\int_\XM k(x, y)\exp\left(\frac{\bar f(x)}{\gamma}\right)\dB\kappa(x)} - \frac{\int_\XM k(x, y)\exp\left(\frac{\bar f(x)}{\gamma}\right)\bar g(x)\dB\kappa'(x)}{\int_\XM k(x, y)\exp\left(\frac{\bar f(x)}{\gamma}\right)\dB\kappa(x)}\|_\infty.
	\end{align*}
	We now bound these two terms individually.
	For the first term, we have
	\begin{align*}
		&\ \|\frac{\int_\XM k(x, y)\exp\left(\frac{\bar f(x)}{\gamma}\right)\bar g(x)\dB\kappa(x)}{\int_\XM k(x, y)\exp\left(\frac{\bar f(x)}{\gamma}\right)\dB\kappa(x)} - \frac{\int_\XM k(x, y)\exp\left(\frac{\bar f(x)}{\gamma}\right)\bar g(x)\dB\kappa(x)}{\int_\XM k(x, y)\exp\left(\frac{\bar f(x)}{\gamma}\right)\dB\kappa'(x)}\|_\infty\\
		\leq&\ \|\int_\XM k(x, y)\exp\left(\frac{\bar f(x)}{\gamma}\right)\bar g(x)\dB\kappa(x)\|_\infty\|\frac{\int_\XM k(x, y)\exp\left(\frac{\bar f(x)}{\gamma}\right)\left[\dB\kappa(x) - \dB\kappa'(x)\right]}{\int_\XM k(x, y)\exp\left(\frac{\bar f(x)}{\gamma}\right)\dB\kappa(x)\int_\XM k(x, y)\exp\left(\frac{\bar f(x)}{\gamma}\right)\dB\kappa'(x)}\|_\infty\\
		=&\ \OM(\|\bar g\|_\infty\cdot d_{bl}(\kappa, \kappa')).
	\end{align*}
	For the second term, we bound
	\begin{align*}
		&\ \|\frac{\int_\XM k(x, y)\exp\left(\frac{\bar f(x)}{\gamma}\right)\bar g(x)\dB\kappa(x)}{\int_\XM k(x, y)\exp\left(\frac{\bar f(x)}{\gamma}\right)\dB\kappa(x)} - \frac{\int_\XM k(x, y)\exp\left(\frac{\bar f(x)}{\gamma}\right)\bar g(x)\dB\kappa'(x)}{\int_\XM k(x, y)\exp\left(\frac{\bar f(x)}{\gamma}\right)\dB\kappa(x)}\|_\infty\\ 
		\leq&\ \|\frac{\int_\XM k(x, y)\exp\left(\frac{\bar f(x)}{\gamma}\right)\bar g(x)[\dB\kappa(x) - \dB\kappa'(x)]}{\int_\XM k(x, y)\exp\left(\frac{\bar f(x)}{\gamma}\right)\dB\kappa(x)} \|_\infty = \OM(\|\bar g\|_\infty\cdot d_{bl}(\kappa, \kappa')). 
	\end{align*}
	Combining the above inequalities, we have
	\begin{equation} \label{eqn_proof_bound_3}
		\|d^1_{\bar g}\AM(\bar f, \kappa) - d^1_{\bar g}\AM(\bar f, \kappa')\|_\infty = \OM(\|\bar g\|_\infty\cdot d_{bl}(\kappa, \kappa')).
	\end{equation}
	We are now ready to bound $\textcircled{3}$: 
	Denote $g = d^1_hf_{\theta, \mu'}$, $\alpha = {T_\theta}_\sharp\mu$, $\alpha' = {T_\theta}_\sharp\mu'$, $f = \AM[f_{\theta, \mu'}, \alpha]$ and $f' = \AM[f_{\theta, \mu'}, \alpha']$.
	From the chain rule of the Gateaux derivative, we compute
	\begin{align*}
		\textcircled{3} =&\ \big\|d^1_{d^1_g\AM[f_{\theta, \mu'}, \alpha]}\AM[f, \beta] - d^1_{d^1_g\AM[f_{\theta, \mu'}, \alpha']}\AM[f', \beta]\big\|_\infty\\
		\leq&\ \big\|d^1_{d^1_g\AM[f_{\theta, \mu'}, \alpha]}\AM[f,\beta] - d^1_{d^1_g\AM[f_{\theta, \mu'}, \alpha']}\AM[f, \beta]\big\|_\infty
		+ \big\|d^1_{d^1_g\AM[f_{\theta, \mu'}, \alpha']}\AM[f, \beta] - d^1_{d^1_g\AM[f_{\theta, \mu'}, \alpha']}\AM[f', \beta]\big\|_\infty.
	\end{align*}
	We now bound these two terms individually.\\
	For the first term, use \eqref{eqn_contraction_of_A} to derive
	\begin{equation*}
		\big\|d^1_{d^1_g\AM[f_{\theta, \mu'}, \alpha]}\AM[f,\beta] - d^1_{d^1_g\AM[f_{\theta, \mu'}, \alpha']}\AM[f, \beta]\big\|_\infty \leq 2\lambda \|d^1_g\AM[f_{\theta, \mu'}, \alpha] - d^1_g\AM[f_{\theta, \mu'}, \alpha']\|_\infty = \OM(\|g\|_\infty\cdot d_{bl}(\mu, \mu')),
	\end{equation*}
	where we use \eqref{eqn_proof_bound_3} in the second equality.\\
	For the second term, use \eqref{eqn_proof_bound_2} to derive
	\begin{equation*}
		\big\|d^1_{d^1_g\AM[f_{\theta, \mu'}, \alpha']}\AM[f, \beta] - d^1_{d^1_g\AM[f_{\theta, \mu'}, \alpha']}\AM[f', \beta]\big\|_\infty = \OM(\|d^1_g\AM[f_{\theta, \mu'}, \alpha']\|_\infty\cdot d_{bl}(\mu, \mu')) = \OM(\|g\|_\infty\cdot d_{bl}(\mu, \mu')),
	\end{equation*}
	where we use \eqref{eqn_proof_bound_0} in the last equality.\\
	Combing the above two results, we have 
	\begin{equation}
		\textcircled{3} = \OM(\|g\|_\infty\cdot d_{bl}(\mu, \mu')) = \OM(d_{bl}(\mu, \mu'))
	\end{equation}
	since $\|g\|_\infty = \|d^1_hf_{\theta, \mu'}\|_\infty$ is bounded.
	\subsection{Bounding \textcircled{4}}
	In this section, we slightly abuse the notation and denote $\AM(f, \theta, \mu) = \AM(f, {T_\theta}_\sharp\mu)$, where dependence on $\theta$ is made explicit.
	Use the chain rule of Gateaux derivative to compute
	\begin{equation}
		d_h^2\BM[f, \theta, \mu] = d^1_{d^2_h \AM(f, \theta,\mu)} \AM(\AM(f, \theta,\mu), \beta).
	\end{equation}
	Besides the direction $d^2_h \AM(f, \theta,\mu)$ can be computed by
	\begin{equation}
		d^2_h \AM(f, \theta,\mu) = \frac{\int_\XM \exp\left(\frac{-c(T_\theta(x), y) + f(T_\theta(x))}{\gamma}\right) \langle J^\top_{T_\theta(x)}\left[-\nabla_1 c(T_\theta(x), y) + \nabla f(T_\theta(x))\right], h\rangle\dB\mu(x)}{\int_\XM \exp\left(\frac{-c(T_\theta(x), y) + f(T_\theta(x))}{\gamma}\right) \dB\mu(x)},
	\end{equation}
	where $J_{T_\theta(x)}$ denotes the Jacobian matrix of $T_\theta(x)$ with respect to $\theta$.
	Denote $l_1(x, y) = \exp\left(\frac{-c(T_\theta(x), y) + f(T_\theta(x))}{\gamma}\right)$ and $l_2(x, y) = J^\top_{T_\theta(x)}\left[-\nabla_1 c(T_\theta(x), y) + \nabla f(T_\theta(x))\right]$.
	Using this expression of $d^2_h \AM(f, \theta,\mu)$, we can bound
	\begin{align*}
		&\ \|d^2_h \AM(f, \theta,\mu) - d^2_h \AM(f, \theta,\mu')\|_\infty \\
		\leq&\ \big\|\frac{\int_\XM l(x, y) l_2(x, y)\dB\mu(x)}{\int_\XM l(x, y) \dB\mu(x)} - \frac{\int_\XM l(x, y) l_2(x, y)\dB\mu'(x)}{\int_\XM l(x, y) \dB\mu'(x)}\big\|_\infty\cdot\|h\|_\infty \\
		\leq&\ \big\|\frac{\int_\XM l(x, y) l_2(x, y)\dB\mu(x)}{\int_\XM l(x, y) \dB\mu(x)} - \frac{\int_\XM l(x, y) l_2(x, y)\dB\mu'(x)}{\int_\XM l(x, y) \dB\mu(x)}\big\|_\infty\cdot\|h\|_\infty \\
		&\ + \big\|\frac{\int_\XM l(x, y) l_2(x, y)\dB\mu'(x)}{\int_\XM l(x, y) \dB\mu(x)} - \frac{\int_\XM l(x, y) l_2(x, y)\dB\mu'(x)}{\int_\XM l(x, y) \dB\mu'(x)}\big\|_\infty\cdot\|h\|_\infty \\
		\leq&\ \big\|\frac{\int_\XM l(x, y) l_2(x, y)\left[\dB\mu(x) - \dB\mu'(x)\right]}{\int_\XM l(x, y) \dB\mu(x)}\big\|_\infty\cdot\|h\|_\infty\\
		&\ + \|\int_\XM l(x, y) l_2(x, y)\dB\mu'(x)\|_\infty\big\|\frac{\int_\XM l(x, y) [\dB\mu'(x) -  \dB\mu(x)]}{\int_\XM l(x, y) \dB\mu(x)\int_\XM l(x, y) \dB\mu'(x)}\big\|_\infty\cdot\|h\|_\infty\\
		=&\ \OM(d_{bl}(\mu, \mu')).
	\end{align*}
	We are now ready to bound \textcircled{4}. First, we can bound \textcircled{4} as
	\begin{align*}
	\textcircled{4} = &\ \|d^1_{d^2_h \AM(f, \theta,\mu)} \AM(\AM(f, \theta,\mu), \beta) - d^1_{d^2_h \AM(f, \theta,\mu')} \AM(\AM(f, \theta,\mu'), \beta)\|_\infty\\
	\leq&\ \|d^1_{d^2_h \AM(f, \theta,\mu)} \AM(\AM(f, \theta,\mu), \beta) - d^1_{d^2_h \AM(f, \theta,\mu')} \AM(\AM(f, \theta,\mu), \beta)\|_\infty \\
	&\ + \|d^1_{d^2_h \AM(f, \theta,\mu')} \AM(\AM(f, \theta,\mu), \beta) - d^1_{d^2_h \AM(f, \theta,\mu')} \AM(\AM(f, \theta,\mu'), \beta)\|_\infty.
	\end{align*}
	For the first term, use \eqref{eqn_contraction_of_A} to bound
	\begin{align*}
		\|d^1_{d^2_h \AM(f, \theta,\mu)} \AM(\AM(f, \theta,\mu), \beta) - d^1_{d^2_h \AM(f, \theta,\mu')} \AM(\AM(f, \theta,\mu), \beta)\|_\infty &\ \leq 2\lambda\cdot\|d^2_h \AM(f, \theta,\mu) - d^2_h \AM(f, \theta,\mu')\|_\infty\\
		&\ = \OM(d_{bl}(\mu, \mu')).
	\end{align*}
	For the second term, use \eqref{eqn_proof_bound_2} to bound
	\begin{align*}
		&\ \|d^1_{d^2_h \AM(f, \theta,\mu')} \AM(\AM(f, \theta,\mu), \beta) - d^1_{d^2_h \AM(f, \theta,\mu')} \AM(\AM(f, \theta,\mu'), \beta)\|_\infty\\
		=&\ \OM(\|d^2_h \AM(f, \theta,\mu')\|_\infty\cdot\|\AM(f, \theta,\mu) - \AM(f, \theta,\mu')\|_\infty)\\
		=&\ \OM(d_{bl}(\mu, \mu')).
	\end{align*}
	Altogether, we have $\textcircled{4} = \OM(d_{bl}(\mu, \mu'))$.
%	\section{Convergence of the Sinkhorn-Knopp Algorithm} \label{appendix_convergence_sinkhorn_knopp}
\section{Proof of Proposition \ref{proposition_invariance}} \label{section_proof_proposition_invariance}
Our goal is to show that the continuous-time limit of $\Phi(\theta_s)$ satisfies the same differential equation as $\phi_s$ provided that $\Phi(\theta_0) = \phi_0$.
To do so, first compute the differential equation of $\dot{\Phi(\theta_s)}$
\begin{equation}
	\dot{\Phi(\theta_s)} = - J_{\Phi}(\theta_s) \HB(\theta_s)^{-1}\nabla F(\theta_s),
\end{equation}
where $J_{\Phi}(\theta_s)$ is the Jacobian matrix of $\Phi(\theta)$ at $\theta = \theta_s$.
We then compute the differential equation of $\phi_s$
\begin{align}
	\dot \phi_s &\ = -\left[\nabla^2_\phi \SM(\alpha_{\Phi^{-1}(\phi)}, \alpha_{\Phi^{-1}(\phi_s)})_{\vert \phi = \phi_s}\right]^{-1} \nabla_\phi F(\Phi^{-1}(\phi))_{\vert \phi = \phi_s}\notag\\
	&\ = -\left[J_{\Phi^{-1}}(\phi_s)^\top \nabla^2_\theta \SM(\alpha_\theta, \alpha_{\theta^s})_{\vert \theta = \theta_s} J_{\Phi^{-1}}(\phi_s)\right]^{-1} J_{\Phi^{-1}}(\phi_s)^\top \nabla F(\theta)_{\vert \theta = \theta_s} \label{eqn_appendix_invariance_proof_1}\\
	&\ = - \left[J_{\Phi^{-1}}(\phi_s)\right]^{-1} \nabla^2_\theta \SM(\alpha_\theta, \alpha_{\theta^s})_{\vert \theta = \theta_s} \nabla F(\theta)_{\vert \theta = \theta_s} \notag\\
	&\ = - J_{\Phi}(\theta_s) \HB(\theta_s)^{-1}\nabla F(\theta_s) \label{eqn_appendix_invariance_proof_2}\\
	&\ = \dot{\Phi(\theta_s)}.\notag
\end{align}
Here in \eqref{eqn_appendix_invariance_proof_1}, we use Lemma \ref{?} and in \eqref{eqn_appendix_invariance_proof_2}, we use $\Phi^{-1}(\phi_s) = \theta_s$ and the inverse function theorem $J_{\Phi}(\theta_s)= \left[J_{\Phi^{-1}}(\phi_s)\right]^{-1}$.
\begin{lemma}\label{lemma_appendix_invariance}
	\begin{equation}
		\nabla^2_\phi \SM(\alpha_{\Phi^{-1}(\phi)}, \alpha_{\Phi^{-1}(\phi_s)})_{\vert \phi = \phi_s} = J_{\Phi^{-1}}(\phi_s)^\top \nabla^2_\theta \SM(\alpha_\theta, \alpha_{\theta^s})_{\vert \theta = \theta_s} J_{\Phi^{-1}}(\phi_s)
	\end{equation}
\end{lemma}
\begin{proof}
	content...
\end{proof}
